# Supplementary material for: Structure diagram of binary Lennard-Jones clusters
Source: arXiv:1710.00400 source file (2017-10-01)
Supplement: Supplementary file 1 [file sm.pdf]

# Structure diagram of binary Lennard Jones clusters - Supplemental Material

Marko Mravlak,[1] Thomas Kister,[2] Tobias Kraus,[2] and Tanja Schilling[1]

[1] *Research Unit for Physics and Materials Science, Université du Luxembourg, L-1511 Luxembourg, Luxembourg*

[2] *INM — Leibniz Institute for New Materials, Campus D2 2, 66123 Saarbrücken, Germany*

(Date: January 19, 2016)

## ADDITIONAL PARAMETERS AND OBSERVABLES

Minimal energy structures of binary Lennard-Jones clusters were calculated for different values of van der Waals attractions between B species and between A and B species of particles. A summary of parameters used in the studied models is shown in the table I.

| | $\epsilon_{\rm AA}$ | $\epsilon_{\rm BB}$ | $\epsilon_{\rm AB}$ | $\sigma_{\rm AA}$ | $\sigma_{\rm BB}$ | $\sigma_{\rm AB}$ |
|---|---|---|---|---|---|---|
| model 1 | 1 | 0.01 | 0.10 | 1 | 1 | 1 |
| model 2 | 1 | 0.50 | 0.71 | 1 | 1 | 1 |
| model 3 | 1 | 0.90 | 0.95 | 1 | 1 | 1 |
| model 4 | 1 | 0.62 | 0.31 | 1 | 1 | 1 |
| model 5 | 1 | 0.62 | 0.62 | 1 | 1 | 1 |
| model 6 | 1 | 0.62 | 0.79 | 1 | 1 | 1 |

Table I. Parameters used in the binary Lennard-Jones model to study different combinations of dissimilar materials.

In the first three models the ratio of the intra-species attraction parameter $\epsilon_{\rm BB}$ is varied to describe materials with various degrees of dissimilarity while the inter-species attraction parameter, i.e. the mixing parameter $\epsilon_{\rm AB}$, was calculated using a geometric mean, $\epsilon_{\rm AB} = (\epsilon_{\rm AA}\epsilon_{\rm BB})^{1/2}$. This approximations is also known as the Berthelot combining rule and is commonly used to describe cross interactions in binary mixtures.

To observe the effect of the choice of the mixing attraction on the structure of clusters other values of the mixing parameter were used in the last three models, i.e. $\epsilon_{\rm AB} = \epsilon_{\rm BB}/2$ (model 4), $\epsilon_{\rm AB} = \epsilon_{\rm BB}$ (model 5) and a geometric mean (model 6). Model 4 describes the case of disfavored mixing, for example when two less cross compatible ligands are attached to different nanoparticle types. Here the core-shell structures are not formed but instead we get the Janus-type phase separated clusters.

The results are shown in figures S1, S2, S3, S4 and S5 where we present diagrams of various observables that characterize the structure of the clusters. In addition to the distance of the innermost particle from the center of mass of the cluster in figure S1, the classification of clusters according to the bond order parameters $q_4$ and $q_6$ in figure S2 and the magnitude of the dipole moment in figure S3 we also present two additional observables.

An indication of core-shell structures is the difference $\Delta r_{AB}$ between the average distances $\overline{r}_i$ of the centers of A and B type particles from the centre of mass of the cluster,

$$\Delta r_{AB} = \frac{1}{N_A}\sum_{i=1}^{N_A} r_i^A - \frac{1}{N_B}\sum_{i=1}^{N_B} r_i^B \ , \tag{S1}$$

where $N_A$ and $N_B$ are numbers of A and B type particles. This is shown in figure S4 where we can see that we always obtain core-shell separated clusters except for the models 4 and 5 where mixing of A and B particles is disfavored.

We also show bond-orientational order parameter $w_4$ in figure S5 which is an averaged version of Steinhardt order parameter $q_4$ and which we also used in the cluster classification scheme [S1].

## MINIMIZATION ALGORITHM

To minimize the energy of clusters we use a basinhopping global minimization algorithm with positional and combinatorial local optimization implemented in GMIN program [S2–S5].

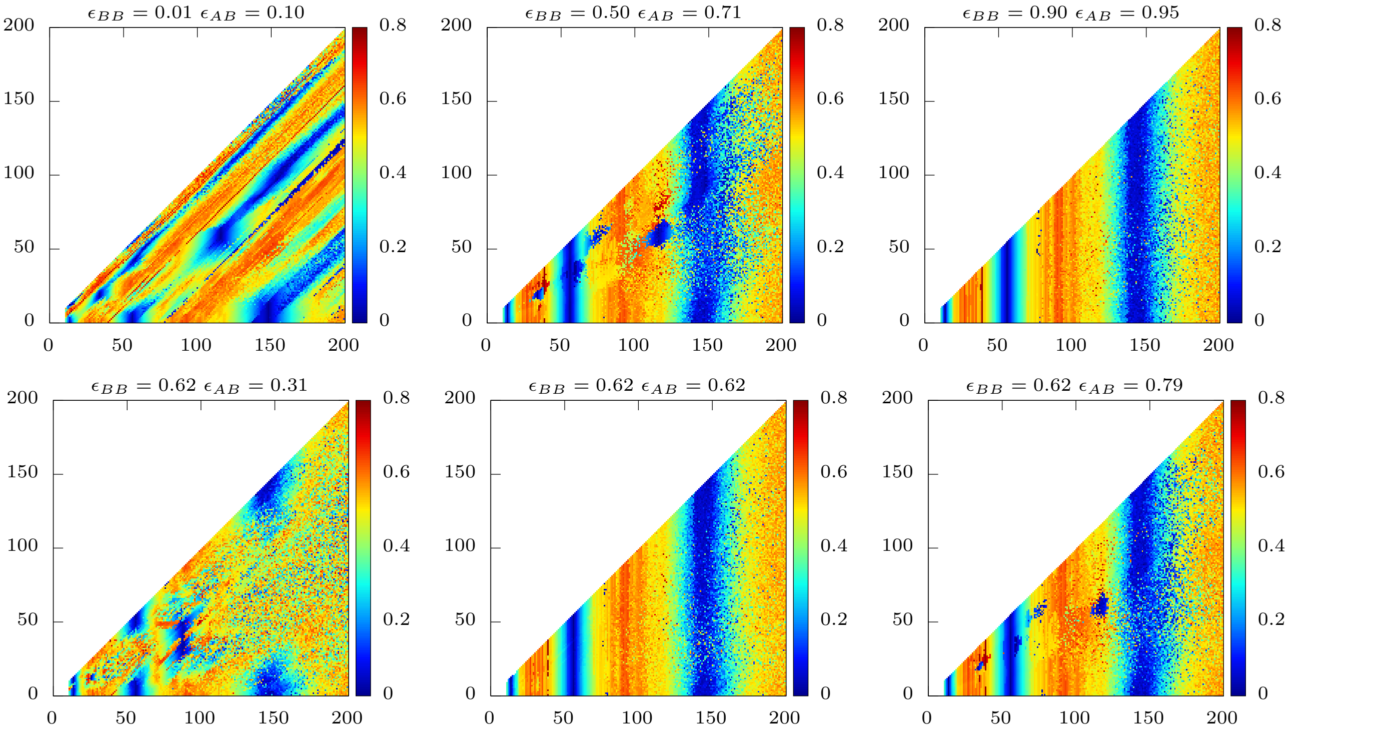


Figure S1. Distance (in units of $\sigma_{AA}$) of the innermost particle from the center of mass of the cluster as a function of cluster composition and size.

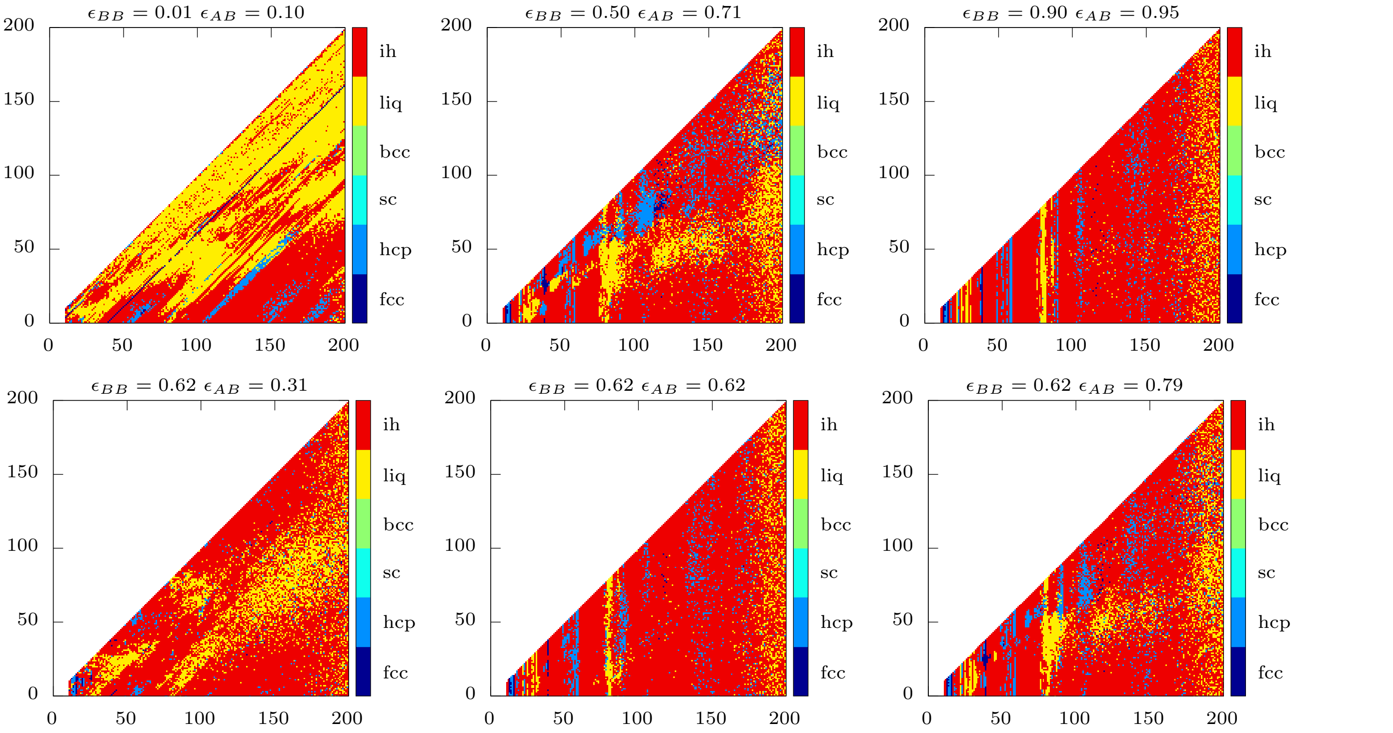


Figure S2. Classification of clusters with different sizes and compositions according to the bond order parameters $q_4$ and $q_6$ averaged over all the particles in the cluster.

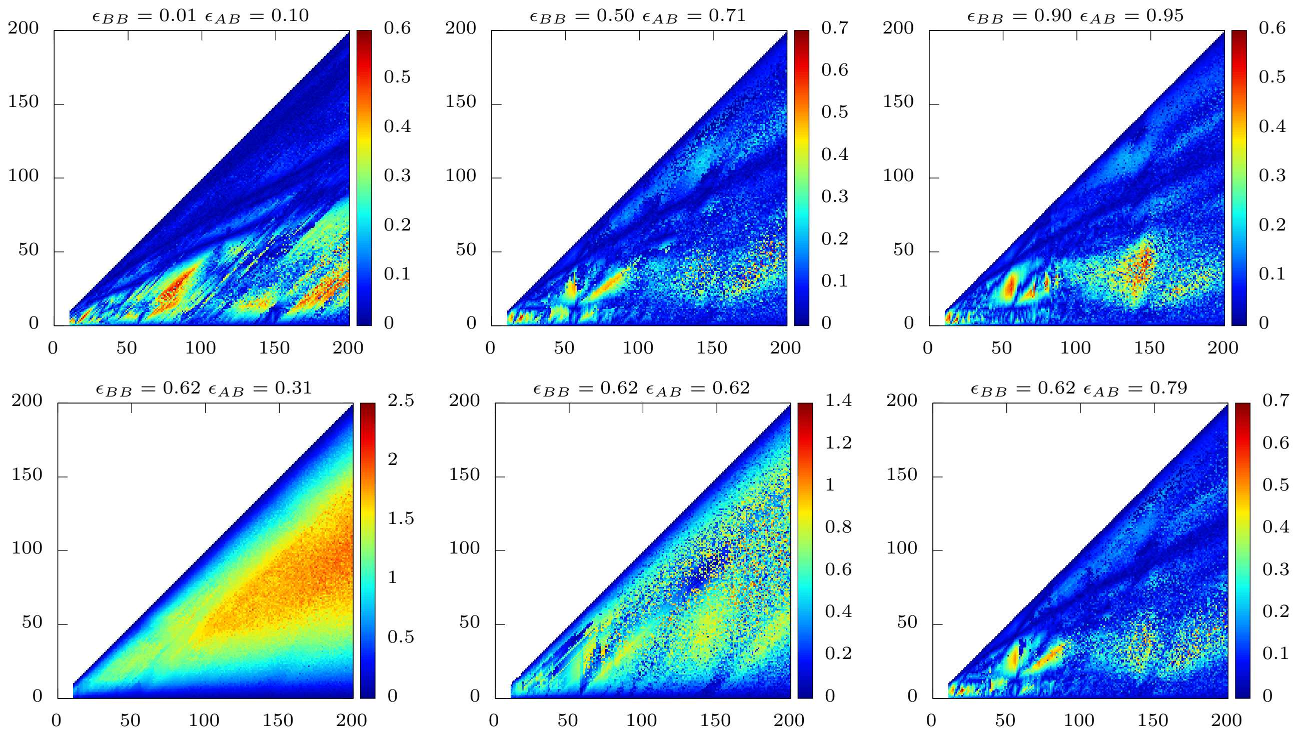


Figure S3. Magnitude of the dipole moment normalized to the number of particles as a function of cluster composition and size. When computing the dipole moment we assigned charge +1 to particles of type A and charge −1 to particles of type B.

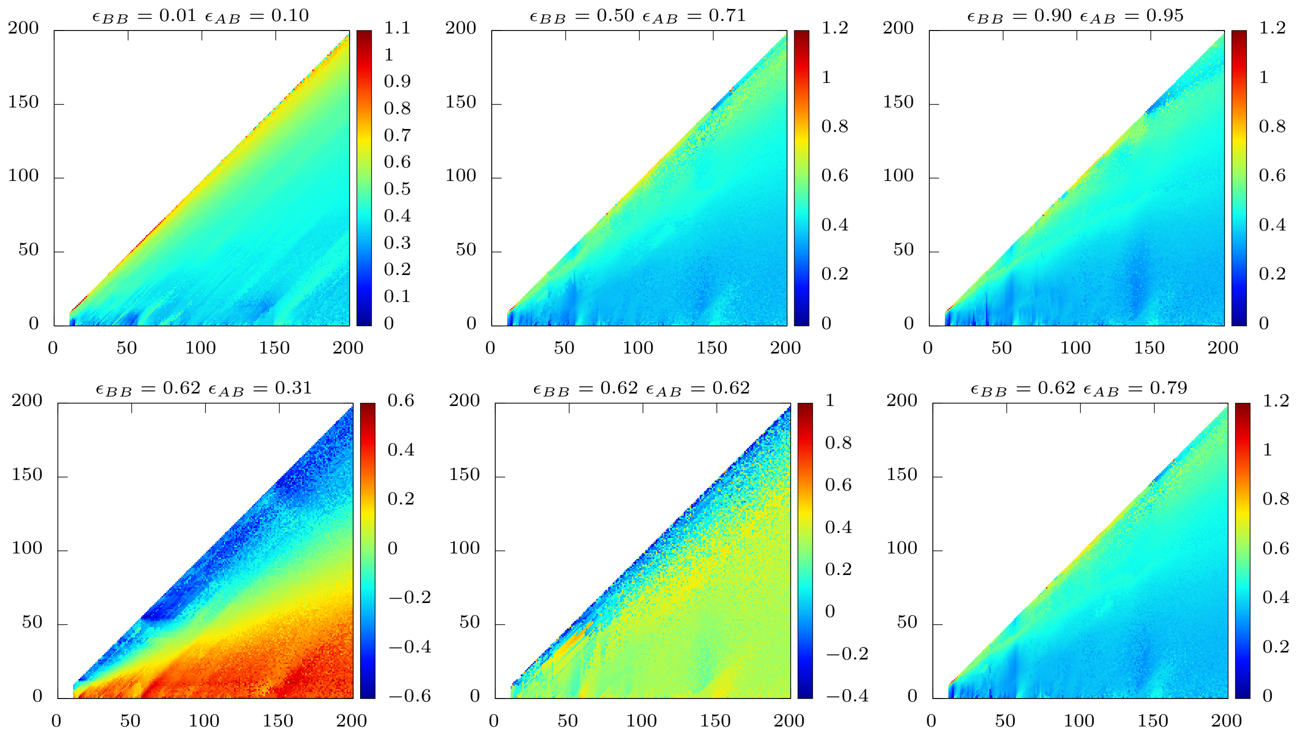


Figure S4. Difference between average distances of A and B type particles from the center of the cluster as a function of cluster composition and size.

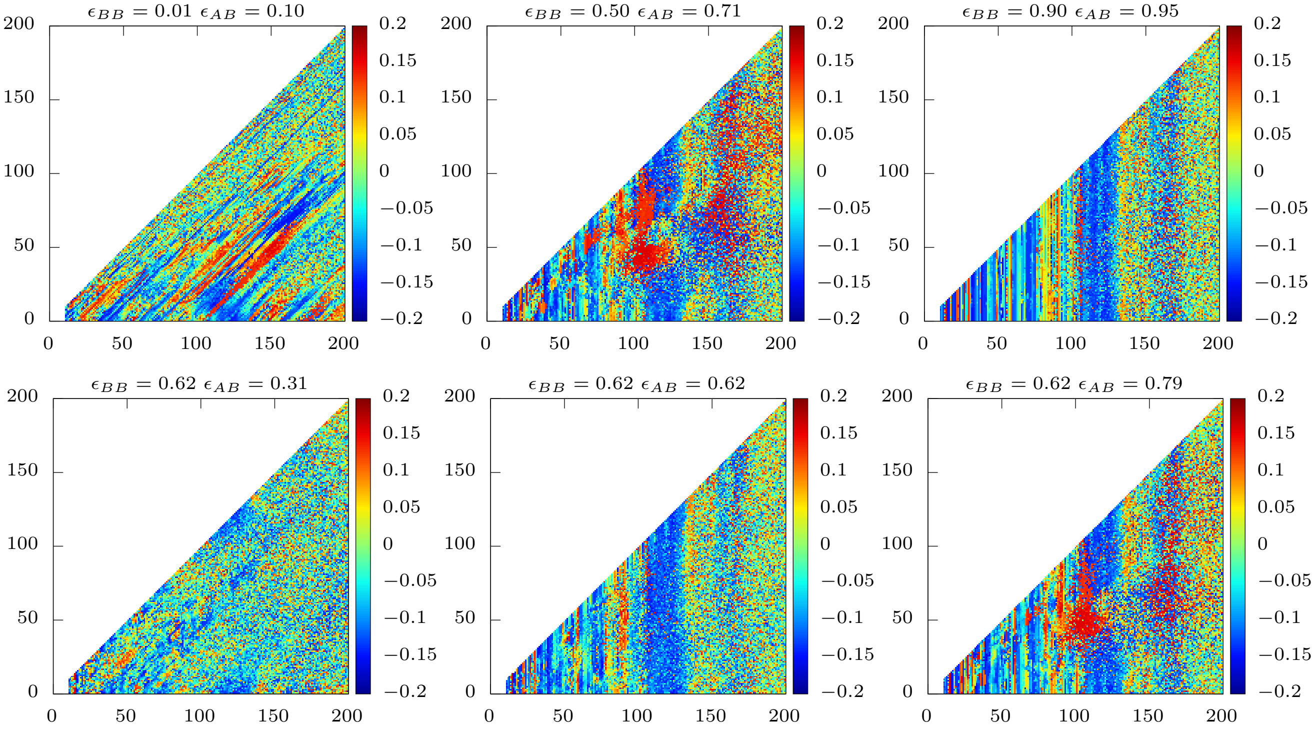


Figure S5. Bond-orientational order parameter $w_4$ as a function of cluster composition and size.

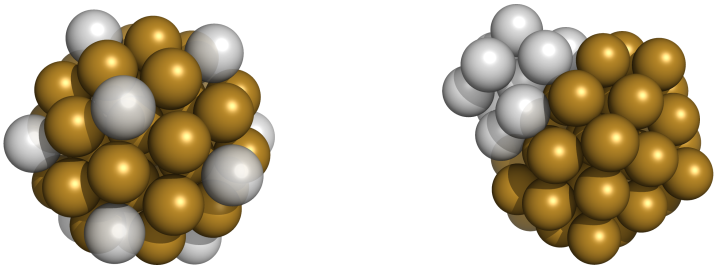

Figure S6. The ideal icosahedron with valency 12 is a minimal energy solution for model 6 for $N = 55$ and $N_B = 12$ (left). The corresponding minimal energy solution for model 4 shows the separation of both particle types (right).

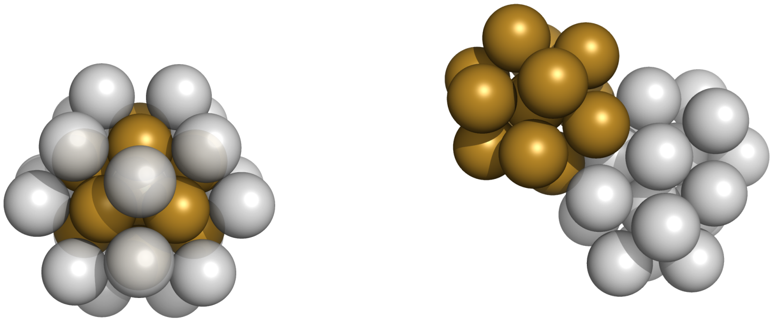

Figure S7. The ideal icosahedron in the core is surrounded by 20 particles of B type at the centers of its 20 triangles in the minimal energy solution for model 6 for $N = 33$ and $N_B = 20$ (left). The corresponding minimal energy solution for model 4 shows the separation of both particle types where particles of A type form a complete icosahedron (right).

We use basin-hopping Monte-Carlo runs of $3 \cdot 10^5$ steps while the temperature is kept fixed at $T = 0.1$. In the Monte-Carlo moves we limited the maximum change of any Cartesian coordinate and imposed a tolerance on the binding energy of individual atoms below which an angular step is taken for that atom. We reseed runs if the energy does not decrease within a certain number of steps. The local optimizations or quenches in the coordinate space are done with the limited-memory BFGS algorithm where the maximum number of iterations allowed is $2 \cdot 10^3$ for the 'sloppy' quenches of the basin-hopping run and $2 \cdot 10^6$ to the final quenches that are used to produce the output. The convergence criterion for the RMS force in the basin-hopping quenches was set to $5 \cdot 10^{-4}$. Quench minima are only considered to be different if their energies differ by at least $10^{-5}$. The tolerance for the RMS force in the final set of quenches that are used to produce the output for file lowest is $10^{-7}$. We calculate the energy of the binary Lennard-Jones clusters without using a distance cutoff. The system is translated so that the centre-of-mass lies at the origin after every quench. We use the container that prevents particles evaporating during quenches. Algorithm also performs homotop refinement for a binary system using an iterated local search (ILS). The refinement happens every basin-hopping step, after the coordinates have been perturbed and quenched. It involves exchanging the coordinates of two unlike atoms until a termination condition is met.

## CLASSIFICATION SCHEME

Steinhardt bond-orientational order parameters $q_4$, $q_6$ and their averaged versions $w_4$, $w_6$ were calculated and averaged over all the bonds in a cluster [S6]. The resulting four values attached to each cluster were then compared to the values of four ideal lattices (SC, BCC, FCC, HCP), to a liquid configuration and to values of complete Mackay icosahedra [S1]. We classify clusters according to the closest matching to these the reference values.

[S1] Y. Wang, S. Teitel, and C. Dellago, J. Chem. Phys. **122**, 214722 (2005).
[S2] D. J. Wales and J. P. K. Doye, J. Phys. Chem. A **101**, 5111 (1997).
[S3] D. Schebarchov and D. J. Wales, J. Chem. Phys. **139**, 221101 (2013).
[S4] D. Schebarchov and D. J. Wales, Phys. Rev. Lett. **113**, 156102 (2014).
[S5] T. V. Bogdan, D. J. Wales, and F. Calvo, J. Chem. Phys. **124**, 044102 (2006).
[S6] P. J. Steinhardt, D. R. Nelson, and M. Ronchetti, Phys. Rev. B **28**, 784 (1983).
